# Supplementary material for: Entanglement-assisted tunneling dynamics of impurities in a double well immersed in a bath of lattice trapped bosons
Source: arXiv:1909.00998 source file (2020-02-13)
Supplement: Supplementary file 1 [file appendix_old.tex]

\appendix

\section{Tunneling dynamics for smaller tilting strength}

\begin{figure*}[]
	\centering
	\includegraphics[scale=0.6]{\pathFigure/gpop_multi_MB_scan11_d0_005.png}
	\caption{(a)-(d) One-body density of the impurity and (e)-(h) one-body density of the majority species using a tilting strength of $\alpha/E_Rk_0^{-1}=0.01$ and employing full many-body calculations. The results in each column correspond to the same interspecies interaction strength $g_{AB}$, ordered from left to right with $g_{AB}/E_rk_0^{-1}=0.2,1.0,2.0,4.0$.}
	\label{fig:MB_densities_small_tilt}
\end{figure*}

In the following we want to demonstrate that a certain minimal tilting strength $\alpha$ is necessary for observing the tunneling dynamics as in Figure \ref{fig:MB_densities} , for which we set $\alpha/E_Rk_0^{-1}=0.1$.
%
In Figure \ref{fig:MB_densities_small_tilt} we show the temporal evolution of (a)-(d) the one-body densities of the impurity and (e)-(h) the majority species using a tilting strength of $\alpha/E_Rk_0^{-1}=0.01$, employing full many-body calculations. Analogously to the previous discussion, we induce the dynamics by initially tilting the double well $V_B$ of the impurity with a tilting strength $\alpha$ and let the system evolve in time for $\alpha=0$. However, in the present case lowering the initial tilting strength to $\alpha/E_Rk_0^{-1}=0.01$ leads to a smaller initial asymmetry of $V_B$. For small $g_{AB}$, i.e. $g_{AB}/E_rk_0^{-1}=0.2,1.0$, we find a rather regular tunneling of the impurity from the left to the right side of the double $V_B$. Comparing this with the dynamical response of an impurity for an initial tilting strength of $\alpha/E_Rk_0^{-1}=0.1$ [cf. Figure \ref{fig:MB_densities} (b)] we find no material barrier tunneling triggered by the density of the majority species. The difference between the two initial tilting strengths is also evident for larger interspecies interaction strengths, e.g. $g_{AB}/E_rk_0^{-1}=2.0,4.0$. Here, the impurity essentially remains localized throughout the dynamics and does not perform any oscillations. Furthermore, the one-body density of the majority species behaves accordingly and does not exhibit distinctive dynamics either.
%
This leads to the conclusion that we need indeed a sufficiently high initial tilting strength $\alpha$ in order to observe a material barrier tunneling with a subsequent controlled transfer of the impurity to the other side of the double well.



\section{Time-averaged effective potentials in many-body and species mean-field calculations}

\begin{figure}[]
	\centering
	\includegraphics[width=0.5\textwidth]{\pathFigure/avEffPot_run_diff_scan11_16_less.pdf}
	\caption{Absolute of the relative difference between the time-averaged effective potential obtained from the many-body calculation $\overline{V_{\textrm{eff,MB}}^B}$ and the species mean-field calculation $\overline{V_{\textrm{eff,sMF}}^B}$ for different interspecies interaction strengths $g_{AB}$.}
	\label{fig:diff_TAEP_MB_sMF}
\end{figure}

In the following we want to underline the necessity to use a many-body ansatz for the analysis of the system instead of a species mean-field ansatz. As already shown in Figure \ref{fig:MF_densities} the time evolution of the one-body density of the impurity species $\rho_B^{(1)}$ calculated with a species mean field ansatz differs for large interspecies interaction strengths $g_{AB}$ from $\rho_B^{(1)}$ obtained via a many-body calculation [cf. Figure \ref{fig:MB_densities}]. Furthermore, also the one-body densities of the majority species $\rho_A^{(1)}$ depicted in the Figures \ref{fig:MF_densities} and \ref{fig:MB_densities} differ from each other. In the following we want to investigate whether the TAEPs obtained with the many-body calculation differ from the TAEPs obtained with a species mean-field ansatz.
%
Therefore, we show in Figure \ref{fig:diff_TAEP_MB_sMF} the absolute of the relative difference between the TAEP of the many-body calculation $\overline{V_{\textrm{eff,MB}}^B}$ and the TAEP from the species mean-field calculation $\overline{V_{\textrm{eff,sMF}}^B}$. We show the results for the interspecies interaction strengths $g_{AB}/E_rk_0^{-1}=0.2,1.0,2.0$ corresponding to the first three tunneling regimes, where we exclude the fourth regime corresponding to $g_{AB}/E_rk_0^{-1}=4.0$. This is due to the fact that $\rho_A^{(1)}$ in Figure \ref{fig:MF_densities} (d) clearly deviates from $\rho_A^{(1)}$ in Figure \ref{fig:MB_densities} (d) making a comparison redundant. In Figure  \ref{fig:diff_TAEP_MB_sMF}, we find for $g_{AB}/E_rk_0^{-1}=0.2$ no significant deviations between the TAEPs, which is due to the weak contribution of $\rho_A^{(1)}$ due to the rather small interspecies interaction strength $g_{AB}$ and the small difference of the corresponding one-body densities of the majority species. However, for larger $g_{AB}$ the relative difference between $\overline{V_{\textrm{eff,MB}}^B}$ and $\overline{V_{\textrm{eff,sMF}}^B}$ increases. In particular, for the left side of the TAEP, where the impurity is located during the time evolution, we find a strong relative deviation.
%
Concluding, for a correct analysis it is not sufficient to construct the Wannier basis based on the TAEP of the mean-field calculation for further analysis. Instead, it is again important to rely on the full many-body calculations.
